# Supplementary material for: Magnetic Resonance Force Microscopy of paramagnetic electron spins at millikelvin temperatures
Source: arXiv:1105.3395 ancillary file (2011-12-07)
Supplement: Supplementary file 1 [file supplementary_vinanteMRFM.pdf]

# Supplementary Information

## Magnetic Resonance Force Microscopy of paramagnetic spins at millikelvin temperatures

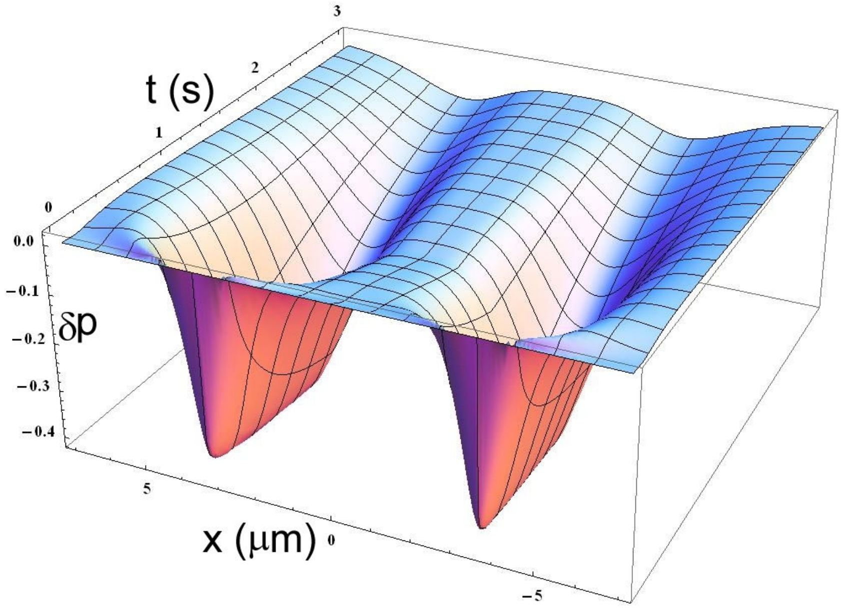


**Supplementary Figure S1. Spatiotemporal evolution of spin polarization.** Numerical simulation of the spatiotemporal evolution of the spin polarization (i.e magnetization normalized to the saturation magnetization), for a set of experimental parameters close to the experimental ones of Fig. 4 of the main paper: $D = 20$ $\mu$m$^2$/s, $D_d = 100$ $\mu$m$^2$/s, $A = 70$ Hz, $T_1 = 1.5$ s, $T = 100$ mK, $B_d = 1.2$ mT. The polarization is expressed as deviation from the thermal equilibrium value, which is also set as initial condition at $t = 0$. Microwave power is switched on at $t = 0$, and off for $t = 1$. The microwave frequency of $f_{\mathrm{rf}} = 2.7$ GHz selects a spin slice centered at $|x_s| = 3.5$ $\mu$m. It can be clearly seen how the microwave-induced depolarization of the resonant slice is rapidly spread, widening the effective slice size to $\approx 3$ $\mu$m during the saturation and recovery transients.

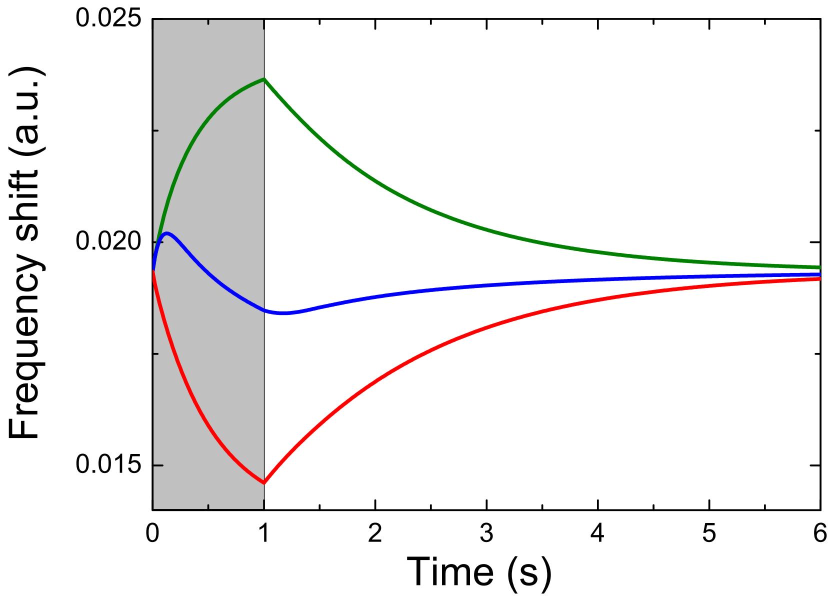


**Supplementary Figure S2. Time evolution of cantilever spring constant.** Numerical simulation of the microwave-induced change of the cantilever spring constant, estimated using Eq. (S4), for the experimental parameters corresponding to Fig. 4 of the main paper. The curves refer respectively to a microwave frequency of 1.25 GHz (green), 2.7 GHz (blue) and 4.2 GHz (red), as in Fig. 4 of main paper. Simulation parameters are the same as in Fig. S1. The shaded region indicates the time in which microwave is on. The qualitative features experimentally observed are substantially reproduced by the simulation, in particular the sign of the induced spring constant change, and the double transient observed at intermediate frequency.

## SUPPLEMENTARY NOTE. NUMERICAL SOLUTIONS OF A SIMPLIFIED MODEL OF SPIN DIFFUSION

In order to do a semi-quantitative estimation of spin diffusion effects in our sample, we have performed a simplified simulation based on the classical equations derived by Genack and Redfield [23] describing spin diffusion in an applied magnetic field gradient:

$$\begin{cases} \frac{\partial M}{\partial t} = D\vec{\nabla}\left(\vec{\nabla}M - \chi_d\vec{\nabla}B\right) \\ \frac{\partial \chi_d}{\partial t} = D_d\nabla^2\chi_d + \frac{\vec{j}\cdot\vec{\nabla}B}{B_d^2} \end{cases} \tag{S1}$$

Here, the two variables are the magnetization $M$ in the external field $B$ generated by the magnet, and the susceptibility of the dipolar bath $\chi_d$. $\vec{j}$ is the magnetization current, characterized in absence of external excitation by the continuity equation $\vec{\nabla}\cdot\vec{j} = -\frac{\partial M}{\partial t}$. $M$ and $\chi_d$ are convenient quantities to express the effective temperature of the Zeeman bath and dipolar bath respectively. While in a constant field the two baths are independent, a field gradient introduces a cross-coupling: in fact two adjacent spins have slightly different Zeeman splitting because of the gradient, so a flip-flop process will not conserve the Zeeman energy. The energy difference has thus to be taken up by the dipolar bath, changing locally the dipolar order. The other parameters appearing in Eqs. (S1) are the Zeeman diffusion constant $D$, the dipolar diffusion constant $D_d$, the position dependent magnetic field $B$ and the mean square value $B_d^2$ of the local field due to neighbouring spins. $D_d$ is expected to be of the same order of magnitude as $D$ [23].

Solutions of Eqs. (S1) are mostly non trivial but in general they follow a two-step behaviour. On a short timescale the second term in the right side of the second of Eqs. (S1) provides an efficient crosscoupling between Zeeman and dipolar bath, bringing quickly the two baths in a local equilibrium condition, for which $\vec{\nabla}M \cong \chi_d\vec{\nabla}B$. This first step can be very fast and will smooth out any strongly ordered initial condition or sharp magnetization gradient, provided that the dipolar order can be rearranged to compensate the required local energy change. On a longer timescale there will be a slower diffusion of the dipolar order, controlled by the diffusion constant $D_d$.

To adapt Eqs. (S1) to our experimental situation we need to make a number of assumptions and approximations. First, the original equations have been derived for a magnetic field with fixed direction, which allows to consider $M$ and $B$ as scalars. This is not strictly true in or case, as the field direction is also changing with position. However, in first approximation we neglect this issue and consider a simple scalar approach. Second, we assume that our system is two-dimensional. Actually, since the resonant slice determined by the microwave field consists of constant $B$ regions, the induced magnetization gradients are always parallel to the field gradient. Therefore, diffusion will proceed mostly in this direction. This suggests to make a further approximation and consider a simple one-dimensional equation, on a direction perpendicular to the resonant slice, for instance the $x$-axis ($y = 0$). Third, we need to model the effect of the microwave saturation process. We do this by adding a term $-A\delta\left(x - |x_s|\right)M\left(x\right)$ in the right-hand side of the $M$ equation. $A$ is the rate of destruction of Zeeman magnetization and according to the Bloch equations it can be estimated as $A \cong \gamma^2 B_1^2 T_2$, while $x_s$ defines the location of the resonant slice. Finally, we model the direct spin-lattice relaxation by adding two equilibration terms in both equations with relaxation time $T_1$. We arrive then at the following simplified equations:

$$\begin{cases} \frac{\partial M}{\partial t} = -D\frac{\partial j}{\partial x} - A\delta\left(x - |x|\right)M - \frac{M - M_{\text{eq}}}{T_1} \\ \frac{\partial \chi_d}{\partial t} = D_d\frac{\partial^2\chi_d}{\partial x^2} + \frac{1}{B_d^2}\frac{\partial B}{\partial x}j - \frac{\chi_d - \chi_{d,\text{eq}}}{T_1} \\ j := -D\left(\frac{\partial M}{\partial x} - \chi_d\frac{\partial B}{\partial x}\right) \end{cases} \tag{S2}$$

with $M = M\left(x,t\right)$ and $\chi_d = \chi_d\left(x,t\right)$ and initial conditions given by the thermal magnetization and susceptibility $M\left(x,0\right) = M_{\text{eq}}$ , $\chi_d\left(x,0\right) = \chi_{d,\text{eq}}$.

The magnetic field corresponding to the experimental condition (field of a dipole $m = 8 \times 10^{-11}$ A/m, oriented along $x$, at a distance $d = 3.6$ $\mu$m from the $x$-axis, and spins probed on the $x$-axis) is given by:

$$B\left(x\right) = B_0\frac{\sqrt{1 + \frac{3x^2}{x^2+d^2}}}{\left(1 + \frac{x^2}{d^2}\right)^{\frac{3}{2}}}. \tag{S3}$$

with $B_0 \approx 170$ mT.

We now estimate the remaining parameters of the simulations. The diffusion constant $D \cong 20$ $\mu$m$^2$/s has been estimated in the main paper. The dipolar diffusion constant $D_d$ is expected to be of the same order of magnitude. However, recent experiments on nuclear spins measured values up to 4-7 times larger [30], in our case this would lead

to an expected value $D_d \cong 100\ \mu\text{m}^2/\text{s}$. The magnetization destruction rate during saturation process is estimated $A \cong 100$ Hz, and it is set to 0 during the recovery. A reasonable estimation of the spin-lattice relaxation time $T_1 \cong 1$ s is deduced by Fig. 5 of the main paper and related considerations.

We simulated Eqs. (S2) using Wolfram Mathematica 7.0. Besides reconstructing the spatiotemporal evolution of $M(x,t)$ and $\chi_d(x,t)$, we can evaluate the qualitative temporal behaviour of the induced spring constant $\Delta k$ and thus the frequency shift. Following the arguments introduced in the main paper, $\Delta k$ is proportional to :

$$\Delta k \propto \int_{-\infty}^{+\infty} -M(x,t)\, \frac{\partial^2 B(x)}{\partial x^2} dx. \tag{S4}$$

We present some representative results in Fig. S1 and Fig. S2. In Fig. S1 we present the spatiotemporal evolution of the magnetization for a set of experimental parameters close to the experimental ones of Fig. 4 of the main paper and $f_{\text{rf}} = 2.7$ GHz. The microwave is on for $0 < t \leq 1$, selecting a resonant slice located at $|x_s| = 3.5\ \mu$m. During the time evolution, the microwave-induced depolarization of resonant spins rapidly diffuses into non-resonant spins widening the effective resonant slice to an effective width of approximately 3 $\mu$m.

In Fig. S2 we present the change induced in the cantilever spring constant by the microwave saturation, estimated using Eq. (S4), for the experimental parameters corresponding to Fig. 4 of the main paper. We can see that the qualitative features experimentally observed are substantially reproduced by the simulation, in particular the sign of the induced spring constant change, and the double transient observed for the intermediate microwave frequency of 2.7 GHz.

## SUPPLEMENTARY REFERENCES

[30] Boutis G.S., Greenbaum D., Cho H., Cory D.G. & Ramanathan C. *Phys. Rev. Lett.* **92**, 137201 (2004).
